# Supplementary material for: On the Nature of Self-Consistency in Density Functional Theory
Source: arXiv:1803.01763 source file (2018-03-05)
Supplement: Supplementary file 1 [file AppendixC.tex]

% Appendix A

\chapter{Contrained Optimisation Approach to Broyden's Methods} % Main appendix title

\label{appB} % For referencing this appendix elsewhere, use \ref{AppendixA}

\lhead{Appendix B. Contrained Optimisation Approach to Broyden's Methods} % This is for the header on each page - perhaps a shortened title

The derivation of the B1 Jacobian update in the main body of text is equivalent to solving the following constrained optimisation problem,
\begin{gather}
\underset{J_{R,n-1} \in S}{\text{minimise}} \text{ } ||J_{R,n} - J_{R,n-1}||_f^2
\end{gather}
where $||.||_f$ is the \textit{Frobenius norm} of a matrix,
\begin{gather}
||A||_f = \sqrt{\sum_{i=1}^m \sum_{j=1}^n |a_{ij}|^2},
\end{gather}
allowing one to formalise the notion of the `closeness' of two matrices \citep{ML}. The set $S = \{ A \text{ } | \text{ }  A \in \mathbb{R}^{k \times k}, A \Delta \rho^{\text{in}}_n = \Delta R_n \}$ imposes the secant condition. In words, one seeks to find the update that minimises the Frobenius norm (difference) of $J_{R,n} - J_{R,n-1}$ subject to the secant condition, which turns out to be Eq$.$ (\ref{b1}). Broyden's `bad' method (B2) -- dubbed `bad' as he himself dismissed it as inferior to B1 in his work -- is simply the same process involved in deriving B1, but instead minimising the Frobenius norm of $J^{-1}_{R,n} - J^{-1}_{R,n-1}$, yielding
\begin{gather}
\label{b2}
J_{R,n}^{-1} =  J_{R,n-1}^{-1} + \frac{\Delta \rho^{\text{in}}_n - J_{R,n-1}^{-1} \Delta R_n }{ |\Delta R_n|^2} \Delta R_n^T.
\end{gather}
