# Supplementary material for: On the Nature of Self-Consistency in Density Functional Theory
Source: arXiv:1803.01763 source file (2018-03-05)
Supplement: Supplementary file 2 [file AppendixD.tex]

% Appendix A

\chapter{Appendix D. Least-squares fitting algorithm} % Main appendix title

\label{AppendixD} % For referencing this appendix elsewhere, use \ref{AppendixA}

\lhead{Appendix D. \emph{Least-squares fitting algorithm}} % This is for the header on each page - perhaps a shortened title

Re-parametrizing the TBM consists of altering TB parameters (in this case, the parameters corresponding to copper atoms) in order to match the TB band structure to an \textit{ab initio} band structure. This can be done by eye, but a more systematic approach will be taken in this thesis by using a least-squares fitting technique. The goal of least-squares fitting is to minimize the sum of the residuals squared,
\begin{align}
S = \sum_i^n r_i^2 \label{eq:D.1} \\
r_i = y_i - f(x_i) \label{eq:D.2}
\end{align}
between the control bands (DFT) and the variable bands (TB).

The key mechanic of a non-linear least squares fitting technique is the minima searching algorithm. Ideally, the algorithm should find the parameter set that gives the global minimum of S (\ref{eq:D.1}). However, in practice, global optimization is a difficult branch of mathematics with a variety of minima searching methods available. A simplistic, genetic algorithm was chosen (Fig. \ref{msa:figD1}); whilst this may not find the optimum solution, only a good fit around the Fermi level is required. \newpage

\begin{figure}[h]
\centering
\includegraphics[scale=0.7]{FlowChart2}
\caption{Flow chart detailing a simple genetic algorithm used to find an adequate minimum of S}
\label{msa:figD1}
\end{figure}
